# Supplementary material for: Modeling Dynamic Hand-Object Interactions with Applications to Human-Robot Handovers
Source: arXiv:2503.04879 source file (2025-03-06)
Supplement: Supplementary file 1 [file X_supp.tex]

\clearpage
\setcounter{page}{1}
\maketitlesupplementary

The supplementary material contains this document and a video. We describe implementation details in \secref{supp:impl} and experimental details in \secref{supp:exp_details}. In \secref{supp:experiments}, we provide additional experiments. We will release all code and pre-trained models.

\section{Implementation Details}
\label{supp:impl}
For training, we use PPO \cite{schulman2017proximal} and follow the implementation provided in~\cite{christen2022dgrasp}. We present an overview of the important parameters and weight values of the reward function in \tabref{tab:params}. 

\input{sections/tables/para_table}

\section{Experimental Details}
\label{supp:exp_details}
\subsection{Dataset}
In our experiments, we use the ARCTIC dataset~\cite{fan2023arctic} and include sequences from all training subjects and the recently released data from the validation subject s05. We exclude the three objects "scissors", "capsule machine", and "phone" from our experiments. "Scissors" is different from all other objects as it cannot be split into a clear base and articulation part and requires in-hand manipulation. "Phone" and "capsule machine" have very small and thin articulation parts which cannot be modeled with our method currently. We then extract hand pose references according to \secref{supp:label_gen}. From these references, we create a 65\%/35\% train/test-split. 
In total, we generate 745 hand pose references for 8 objects from the dataset, with a train/test split of 488/257 hand pose references.

\subsection{Hand Pose Reference Generation}
\label{supp:label_gen}
We now describe the procedure of retrieving hand pose references from motion capture sequences. Since the sequences contain several different interactions of object manipulation, from which a lot of hand pose references could be extracted, we devise heuristics to obtain diverse frames and avoid redundancy. We distinguish between two types of manipulation in this paper: grasping and articulation.

For each sequence, we first remove all frames where none of the hands is in contact with an object. Next, we filter all remaining frames for grasping and articulation. An interaction is determined as grasping if an object is moved from its underlying surface, i.e., if the velocity of the object base $\dot{\textbf{B}}$ is higher than a threshold $\epsilon_v$. On the other hand, if the articulation angle $\omega$ is changed, we deem an interaction as articulation. To avoid redundancy in hand pose reference frames, we make the assumption that the hand pose does not drastically change during one interaction. Hence, we choose one frame per interaction subsequence.

\begin{figure}
  \centering
  \begin{subfigure}{1.0\linewidth}
    \centering
    {\includegraphics[width=0.3\textwidth]{\dir/artigrasp/figures/seqs/grasp_comparison/pd_1.png}
     \includegraphics[width=0.3\textwidth]{\dir/artigrasp/figures/seqs/grasp_comparison/pd_2.png}
     \includegraphics[width=0.3\textwidth]{\dir/artigrasp/figures/seqs/grasp_comparison/pd_3.png}}
    \caption{PD+IK}
  \end{subfigure}
  \hfill
  \begin{subfigure}{1.0\linewidth}
        \centering
    {\includegraphics[width=0.3\textwidth]{\dir/artigrasp/figures/seqs/grasp_comparison/dgrasp_1.png} 
     \includegraphics[width=0.3\textwidth]{\dir/artigrasp/figures/seqs/grasp_comparison/dgrasp_2.png}
     \includegraphics[width=0.3\textwidth]{\dir/artigrasp/figures/seqs/grasp_comparison/dgrasp_3.png}}
    \caption{D-Grasp}
  \end{subfigure}
  \hfill
  \begin{subfigure}{1.0\linewidth}
        \centering
        {\includegraphics[width=0.3\textwidth]{\dir/artigrasp/figures/seqs/grasp_comparison/ours_1.png}
     \includegraphics[width=0.3\textwidth]{\dir/artigrasp/figures/seqs/grasp_comparison/ours_2.png}
     \includegraphics[width=0.3\textwidth]{\dir/artigrasp/figures/seqs/grasp_comparison/ours_3.png}}
    \caption{Ours}
  \end{subfigure}
  \caption{\textbf{Qualitative evaluation of grasping.} When evaluated only on grasping, PD+IK often fails to successfully grasp the object. On the other hand, D-Grasp and ours succeed at the task.}
    \label{fig:arti:comparison_grasp}
\end{figure}

\begin{figure}
  \centering
  \begin{subfigure}{1.0\linewidth}
        \centering
        {\includegraphics[width=0.3\textwidth]{\dir/artigrasp/figures/seqs/arti_comparison/pd_arti_1.png} 
     \includegraphics[width=0.3\textwidth]{\dir/artigrasp/figures/seqs/arti_comparison/pd_arti_2.png}
     \includegraphics[width=0.3\textwidth]{\dir/artigrasp/figures/seqs/arti_comparison/pd_arti_3.png}}
    \caption{PD+IK}
  \end{subfigure}
  \hfill
  \begin{subfigure}{1.0\linewidth}
        \centering
        {\includegraphics[width=0.3\textwidth]{\dir/artigrasp/figures/seqs/arti_comparison/dgrasp_arti_1.png} 
     \includegraphics[width=0.3\textwidth]{\dir/artigrasp/figures/seqs/arti_comparison/dgrasp_arti_2.png}
     \includegraphics[width=0.3\textwidth]{\dir/artigrasp/figures/seqs/arti_comparison/dgrasp_arti_3.png}}
    \caption{D-Grasp}
  \end{subfigure}
  \hfill
  \begin{subfigure}{1.0\linewidth}
        \centering
        {\includegraphics[width=0.3\textwidth]{\dir/artigrasp/figures/seqs/arti_comparison/ours_arti_1.png} 
     \includegraphics[width=0.3\textwidth]{\dir/artigrasp/figures/seqs/arti_comparison/ours_arti_2.png}
     \includegraphics[width=0.3\textwidth]{\dir/artigrasp/figures/seqs/arti_comparison/ours_arti_3.png}}
    \caption{Ours}
  \end{subfigure}
  \caption{\textbf{Qualitative evaluation of articulation.} When evaluated only on articulation, both PD+IK and D-Grasp often fail at the task. On the other hand, our method can articulate the object successfully.}
    \label{fig:arti:comparison_arti}
\end{figure}

\subsection{Grasping and Articulation}
To evaluate grasping, we generate 30 target \sixD object poses for each hand-pose reference. The target positions are sampled within a range of [-0.15m, 0.15m] in x and y directions and [0.15m, 0.45m] for the z direction. The target object orientation is the initial object orientation disturbed with noise in the range of [-0.3rad, 0.3rad] for all rotation axes. To evaluate articulation, we set 5 target joint angles per trial: 0.5rad, 0.75rad, 1.0rad, 1.25rad and 1.5rad. 
% \SC{What is the range for success for both grasping and articulation? Should be added here}

\subsection{Dynamic Object Grasping and Articulation}
For the evaluation of \task, we randomly sample the target articulated object poses $\overline{\mathbf{\Omega}}$, which consists of the target 6D base pose and the target object joint articulation angle. The target base position is sampled within a range of [-0.1m, -0.05m] in x and y directions and 0m in z direction, since the objects should be relocated back onto the table. The target base orientation is the initial object orientation disturbed with noise in the range of [-0.4rad, 0.4rad] for the yaw axis. The target articulation angle is randomly sampled in the range of [0.5rad, 0.6rad].

\subsection{Hand Pose Reconstruction}
In this experiment, we use the pretrained image-based reconstruction model of ARCTIC~\cite{fan2023arctic} to predict hand-object poses from single images. Since their model is trained on the full training set and the test data is not released, we use the validation set (subject s05) to evaluate this experiment. This allows us to do a direct comparison of individual hand pose references from motion capture and image-based predictions. Our evaluation is conducted on 60 hand pose references selected with the heuristics explained in \secref{supp:label_gen}. We retrieve the images at the corresponding timesteps and pass them to the image-based prediction model. 

\begin{figure}
	\centering
\includegraphics[width=0.47\textwidth]{\dir/artigrasp/figures/seqs/individual_seqs/individual.pdf}
\caption{\textbf{Qualitative outputs of our method.} We provide more sequences for grasping and articulation, which are generated by our method with a single pair of hand pose reference label per interaction. Each sequence is shown from left to right.}
\label{fig:arti:more_samples}
\end{figure}

\section{Additional Experiments}
\label{supp:experiments}

% \subsection{Qualitative Evaluation}
We provide additional qualitative comparisons of our method with baselines for grasping and articulation in \figref{fig:comparison_grasp} and \figref{fig:comparison_arti}, respectively. Given a pair of policies (one per hand), our method can generate diverse grasping and articulation sequences across different objects, which is shown in \figref{fig:more_samples}. Please see our \suppl video for more qualitative examples.

\begin{figure*}[th]
	\centering
\includegraphics[width=1.0\textwidth]{sections/figures/seqs/long_demo/long.pdf}

\caption{\textbf{Long sequence with multiple objects.} We show that our method can generate sequences of manipulating multiple objects. (A) Approaching the mixer with the left hand. (B) Grasping the mixer with the left hand. (C) Articulating the mixer with the right hand while the left hand is holding it. (D) Putting the mixer down on the table. (E) Approaching the box with both hands. (F) Grasping the box with both hands. (G) Relocating the box on the table and moving the left hand to the ketchup bottle. (H) Grasping the ketchup bottle with the left hand and opening the box with the right hand. (I) Relocating the ketchup bottle while the box is being held open. (J) Dropping the ketchup bottle into the box. (K) Moving the left hand away from the box. (L) Closing the box with the right hand.}
\label{fig:long_sequence}
\end{figure*}

\begin{figure}
  \centering
  \begin{subfigure}{1.0\linewidth}
    \centering
     {\includegraphics[width=1.0\textwidth]{sections/figures/seqs/unnatural_labels.pdf}}
    \caption{Unnatural hand pose references}
    \label{fig:unnatural_a}
  \end{subfigure}
  \hfill
  \begin{subfigure}{1.0\linewidth}
    \centering
    {\includegraphics[width=1.0\textwidth]{sections/figures/seqs/failure/unnatural.pdf}}
    \caption{Unnatural generated hand poses}
    \label{fig:unnatural_b}
  \end{subfigure}
  \caption{\textbf{Unnatural hand poses} (a) Some of the hand pose references we extract from the ARCTIC dataset contain unnatural hand poses. (b) Our method can output some unnatural hand poses, which can be due to noise in the hand pose references or because of the trade-off in the task objective.}
    
\end{figure}

\subsection{Long Sequence with Multiple Objects}
Our method can generate long motion sequences in environments with multiple objects, which is shown in \figref{fig:long_sequence}. We use a heuristics-based planner to compose the sequences. Learning a high-level planning module to couple the different phases is an interesting direction to explore in the future. Note that while we propose a controlled setting to evaluate the \task~task, the order of manipulations can also be reversed. For example, an object can first be articulated, and then be moved to a different location.

\subsection{Unnatural Poses}
As shown in \figref{fig:unnatural_b}, our method can generate unnatural poses, which we argue occurs because of noisy pose references from \arctic as seen in \figref{fig:unnatural_a}. We find that especially the index finger is often poorly labeled in the data, which translates to our policies. Developing hand pose priors to incentivize natural poses could be one way to mitigate this issue.
